# Supplementary material for: SADA: Semantic adversarial unsupervised domain adaptation for Temporal Action Localization
Source: arXiv:2312.13377 source file (2025-02-22)
Supplement: Supplementary file 1 [file appendix_val_split.tex]

\section{\red{Results validation split}}\label{sec:appendix_val_split}

\begin{table*}[t]
\centering
\footnotesize
\resizebox{\textwidth}{!}{%
\begin{tabular}{c | l | ccccc | c}
\toprule
Scenario & Model & mAP10\% & mAP20\% & mAP30\% & mAP40\% & mAP50\% & Avg \\
\midrule
\multirow{3}{}{\shortstack{B $\rightarrow$ {all \textbackslash B} \\ (EK100 \textbackslash EK55)}} & Actionformer~\cite{zhang2022actionformer} & 28.93 & 27.63 & 25.73 & 22.26 & 16.97 & 24.30 \\
& Tridet~\cite{shi2023tridet} & 36.97 & 35.94 & 33.78 & 28.46 & 22.64 & 31.56 \\
& \red{Ours (source-only)} & 35.13 & 33.25 & 30.73 & 27.22 & 20.36 & 29.34 \\
& \red{Actionformer+SADA~\cite{zhang2022actionformer}} & 33.58 & 32.02 & 29.69 & 25.96 & 20.13 & 28.28 \\
& \red{Tridet+SADA~\cite{shi2023tridet}} & 31.34 & 30.16 & 27.94 & 24.48 & 19.31 & 26.64 \\
& \textbf{Ours (SADA)} & 36.88 & 35.59 & 32.69 & 28.57 & 22.43 & 31.23 \\
\midrule
\multirow{3}{}{\shortstack{B $\rightarrow$ {all \textbackslash B} \\ (EK55)}} & Actionformer~\cite{zhang2022actionformer} & 30.54 & 29.21 & 26.83 & 23.03 & 17.26 & 25.37 \\
& Tridet~\cite{shi2023tridet} & 33.25 & 32.25 & 30.20 & 27.15 & 21.85 & 28.94 \\
& \red{Ours (source-only)} & 33.26 & 32.06 & 29.89 & 27.15 & 20.65 & 28.60 \\
& \red{Actionformer+SADA~\cite{zhang2022actionformer}} & 31.54 & 30.20 & 28.75 & 25.74 & 20.73 & 27.39 \\
& \red{Tridet+SADA~\cite{shi2023tridet}} & 33.25 & 32.25 & 30.20 & 27.15 & 21.85 & 28.94 \\
& \textbf{Ours (SADA)} & 32.90 & 31.69 & 29.93 & 26.70 & 20.66 & 28.37 \\
\midrule
\multirow{3}{}{\shortstack{W $\rightarrow$ {all \textbackslash W} \\ (EK100 \textbackslash EK55)}} & Actionformer~\cite{zhang2022actionformer} & 34.24 & 32.85 & 30.42 & 27.09 & 21.02 & 29.13 \\
& Tridet~\cite{shi2023tridet} & 25.54 & 24.68 & 21.87 & 18.40 & 13.30 & 20.76 \\
& \red{Ours (source-only)} & 24.41 & 22.78 & 20.37 & 18.27 & 13.24 & 19.82 \\
& \red{Actionformer+SADA}\cite{zhang2022actionformer} & 24.67 & 23.42 & 21.38 & 18.91 & 13.67 & 20.41 \\
& \red{Tridet+SADA}\cite{shi2023tridet} & 25.54  & 24.68 & 21.87 & 18.40 & 13.30 & 20.76 \\
& \textbf{Ours (SADA)} & 23.67 & 22.05 & 19.77 & 17.09 & 13.05 & 19.13 \\
\midrule
\multirow{3}{}{\shortstack{W $\rightarrow$ {all \textbackslash W} \\ (EK55)}} & Actionformer~\cite{zhang2022actionformer} & 28.19 & 27.29 & 25.35 & 22.41 & 17.94 & 24.24 \\
& Tridet~\cite{shi2023tridet} & 30.10 & 28.70 & 26.63 & 23.97 & 19.10 & 25.70 \\
& \red{Ours (source-only)} & 29.31 & 27.94 & 26.23 & 23.01 & 18.84 & 25.07 \\
& \red{Actionformer+SADA}\cite{zhang2022actionformer} & 29.35 & 27.80 & 25.76 & 22.80 & 18.53 & 24.85 \\
& \red{Tridet+SADA}\cite{shi2023tridet} & 30.10 & 28.70 & 26.63 & 23.97 & 19.10 & 25.70 \\
& \textbf{Ours (SADA)} & 31.08 & 29.68 & 27.77 & 24.38 & 20.02 & 26.58 \\
\midrule
\midrule
\multirow{3}{}{EK55 $\rightarrow$ (EK100 \textbackslash EK55)} & Actionformer~\cite{zhang2022actionformer} & 23.02 & 21.94 & 20.06 & 17.41 & 13.88  & 19.26 \\
& Tridet~\cite{shi2023tridet} & 40.16 & 38.89 & 35.89 & 29.73 & 22.16 & 33.37 \\
& \red{Ours (source-only)} & 36.44 & 35.14 & 32.32 & 27.23 & 20.24 & 30.27 \\
& \red{Actionformer+SADA}\cite{zhang2022actionformer} & 34.89 & 33.62 & 31.23 & 25.42 & 18.76 & 28.78 \\
& \red{Tridet+SADA}\cite{shi2023tridet} & 40.16 & 38.89 & 35.89 & 29.73 & 22.16 & 33.37 \\
& \textbf{Ours (SADA)} & & & & & & \\
\midrule
\multirow{3}{}{(EK100 \textbackslash EK55) $\rightarrow$ EK55} & Actionformer~\cite{zhang2022actionformer} & 21.47 & 20.57 & 19.09 & 16.89 & 13.69 & 18.34 \\
& Tridet~\cite{shi2023tridet} & 21.57 & 20.54 & 19.40 & 17.72 & 14.44 & 18.73 \\
& \red{Ours (source-only)} & 20.96 & 20.22 & 19.08 & 16.97 & 14.09 & 18.27 \\
& \red{Actionformer+SADA}\cite{zhang2022actionformer} & 20.18 & 19.46 & 18.52 & 16.57 & 13.38 & 17.62 \\
& \red{Tridet+SADA}\cite{shi2023tridet} & 21.57 & 20.54 & 19.40 & 17.72 & 14.44 & 18.73 \\
& \textbf{Ours (SADA)} & & & & & & \\
\bottomrule
\end{tabular}}
\vspace{0.3cm}
\caption{Comparison of our proposal \textit{SADA} with the state-of-the-art for the 4 different appearance-shift scenarios (1-4) and the 2 different acquisition-shift scenarios (5-6) on the \textbf{validation split of the target domain}.}
\label{tab:appendix_charadesego_results}
\end{table*}

\begin{table}[t]
\centering
\footnotesize
\resizebox{0.75\textwidth}{!}{%
\begin{tabular}{c | ccc | c | ccc | c}
& \multicolumn{4}{c|}{\textbf{B $\rightarrow$ {all \textbackslash B} (EK100-EK55)}} & \multicolumn{4}{c}{\textbf{B $\rightarrow$ {all\textbackslash B} (EK55)}} \\
\midrule
\textbf{Model} & \multicolumn{3}{c|}{\textbf{mAP {10,30,50}\%}} & \textbf{Avg} & \multicolumn{3}{c|}{\textbf{mAP {10,30,50}\%}} & \textbf{Avg} \\
\midrule
\textbf{Ours (LB)} & 35.13 & 30.73 & 20.36 & 28.74 & 33.26 & 29.89 & 20.65 & 27.93 \\
\textbf{Ours (UB)} & 40.02 & 35.64 & 26.64 & 34.1 & 32.62 & 30.06 & 23.31 & 28.66 \\
\midrule
\red{ADDA} \cite{} & 37.69 & 33.27 & 22.78 & 31.25 & 32.69 & 29.80 & 20.82 & 27.77 \\
\red{WDGRL} \cite{} & 29.89 & 25.77 & 17.90 & 24.52 & 32.28 & 29.58 & 19.47 & 27.11 \\
DANN \cite{ganin2016domain} & 37.50 & 33.07 & 22.52 & 31.03 & 29.63 & 25.04 & 15.96 & 23.54 \\
Semantic centroids \cite{xie2018learning} & 36.17 & 31.76 & 20.79 & 29.57 & 32.73 & 29.73 & 20.22 & 27.56 \\
SSTDA \cite{chen2020action} & 37.51 & 33.32 & 22.89 & 31.24 & 32.74 & 29.68 & 20.53 & 27.65 \\
\red{TranSVAE} \cite{wei2024unsupervised} & 29.81 & 25.18 & 16.73 & 23.90 & 31.46 & 27.41 & 17.07 & 25.31\\
\midrule
\textbf{Ours (SADA)} & 36.88 & 32.69 & 22.43 & 30.66 & 32.90 & 29.93 & 20.66 & 27.83 \\
\bottomrule
\end{tabular}%
}
\vspace{0.3cm}
\caption{Ablation study on Scenarios 1 and 3, comparing the performance of \textit{SADA} with relevant domain adaptation methods coupled in our proposed architecture to ensure a fair comparison. Evaluated on the \textbf{validation split of the target domain.} }
\vspace{-0.9cm}
\label{tab:ablation_baselines_upper_bounds1}
\end{table}

\begin{table}[t]
\centering
\footnotesize
\resizebox{0.75\textwidth}{!}{%
\begin{tabular}{c | ccc | c | ccc | c}
& \multicolumn{4}{c|}{\textbf{W $\rightarrow$ {all \textbackslash W} (EK100-EK55)}} & \multicolumn{4}{c}{\textbf{W $\rightarrow$ {all\textbackslash W} (EK55)}} \\
\midrule
\textbf{Model} & \multicolumn{3}{c|}{\textbf{mAP {10,30,50}\%}} & \textbf{Avg} & \multicolumn{3}{c|}{\textbf{mAP {10,30,50}\%}} & \textbf{Avg} \\
\midrule
\textbf{Ours (LB)} & 24.41 & 20.37 & 13.24 & 19.34 & 29.31 & 26.23 & 18.84 & 24.79\\
\textbf{Ours (UB)} & & & & & & & & \\
\midrule
\red{ADDA} \cite{} & 22.84 & 19.14 & 12.76 & 18.24 & 31.79 & 28.62 & 20.16 & 26.86  \\
\red{WDGRL} \cite{} & 22.84 & 19.14 & 12.76 & 18.24 & 31.79 & 28.62 & 20.16 & 26.85 \\
DANN \cite{ganin2016domain} & 24.00 & 20.24 & 13.23 & 19.15 & 31.25 & 27.97 & 19.80 & 26.34 \\
Semantic centroids \cite{xie2018learning} & 22.46 & 19.14 & 12.25 & 17.95 & 30.60 & 27.61 & 18.63 & 25.61 \\
SSTDA \cite{chen2020action} & 22.42 & 19.33 & 12.36 & 18.03 & 31.31 & 27.68 & 19.62 & 26.20 \\
\red{TranSVAE} \cite{wei2024unsupervised} & & & & & 23.76 & 20.35 & 12.81 & 18.97 \\
\midrule
\textbf{Ours (SADA)} & 23.67 & 19.77 & 13.05 & 18.83 & 31.08 & 27.77 & 20.02 & 26.29\\
\bottomrule
\end{tabular}%
}
\vspace{0.3cm}
\caption{Ablation study on Scenarios 2 and 4, comparing the performance of \textit{SADA} with relevant domain adaptation methods coupled in our proposed architecture to ensure a fair comparison. Evaluated on the \textbf{validation split of the target domain.} }
\vspace{-0.9cm}
\label{tab:ablation_baselines_upper_bounds2}
\end{table}
